# Supplementary material for: Source of radio emissions induced by the Galilean moons Io, Europa and Ganymede: in situ measurements by Juno
Source: arXiv:2308.05541 source file (2023-08-10)
Supplement: Supplementary file 1 [file SI_Louis_Jovian-moons_in-situ_radio_emission.pdf]

# Supporting Information for " Source of radio emissions induced by the Galilean moons Io, Europa and Ganymede: *in situ* measurements by Juno"

C. K. Louis[1,2,3], P. Louarn[2], B. Collet[4], N. Clément[2,5], S. Al Saati[2,6], J. R. Szalay[7], V. Hue[8], L. Lamy[3,4], S. Kotsiaros[9], W. S. Kurth[10], C. M. Jackman[1], Y. Wang[2,11,12], M. Blanc[2,5], F. Allegrini[13,14], J. E. P. Connerney[15], D. Gershman[16]

[1]School of Cosmic Physics, DIAS Dunsink Observatory, Dublin Institute for Advanced Studies, Dublin 15, Ireland
[2]IRAP, Université de Toulouse, CNRS, CNES, UPS, Toulouse, France
[3]LESIA, Observatoire de Paris, Université PSL, CNRS, Sorbonne Université, Université de Paris Meudon, France
[4]Pythéas, Aix Marseille Université, CNRS, CNES, Marseille, France
[5]Laboratoire d'Astrophysique de Bordeaux, Univ. Bordeaux, CNRS, B18N, Allée Geoffroy Saint-Hilaire, 33615 Pessac, France
[6]CPHT, CNRS, Institut Polytechnique de Paris, Route de Saclay, 91128 Palaiseau, France
[7]Department of Astrophysical Sciences, Princeton University, Princeton, New Jersey, USA
[8]NAix-Marseille Université, CNRS, CNES, Institut Origines, LAM, Marseille, France
[9]Technical University of Denmark: Kgs. Lyngby, Denmark
[10]Department of Physics and Astronomy, University of Iowa, Iowa City, Iowa, USA
[11]State Key Laboratory of Space Weather, National Space Science Center, Chinese Academy of Sciences, Beijing, China
[12]College of Earth and Planetary Sciences, University of Chinese Academy of Sciences, Beijing, China
[13]Southwest Research Institute, San Antonio, Texas, USA
[14]Department of Physics and Astronomy, University of Texas at San Antonio, San Antonio, Texas, USA
[15]NSpace Research Corporation, Annapolis, MD, USA, 21403
[16]NASA Goddard Space Flight Center, Greenbelt, MD, USA

**Contents of this file:**

1. Figures S1 to S5

**Introduction**

This Supporting Information contains figures that complement the figures and text in the main manuscript. Figure S1 complements Figure 1 by providing details of magnetic disturbances. Figure S2 to S4 provides Juno data for the three other Io-induced radio emission source crossings discussed in the text of the main manuscript. Finally, Figure S5 gives details of magnetic disturbances during the Ganymede-induced radio emission source crossing of PJ#20.

**Figure S1 – Magnetic field perturbations from Juno/MAG measurements during Io-induced radio emission source crossing on 2017 March 27 (Perijove #5 South)**

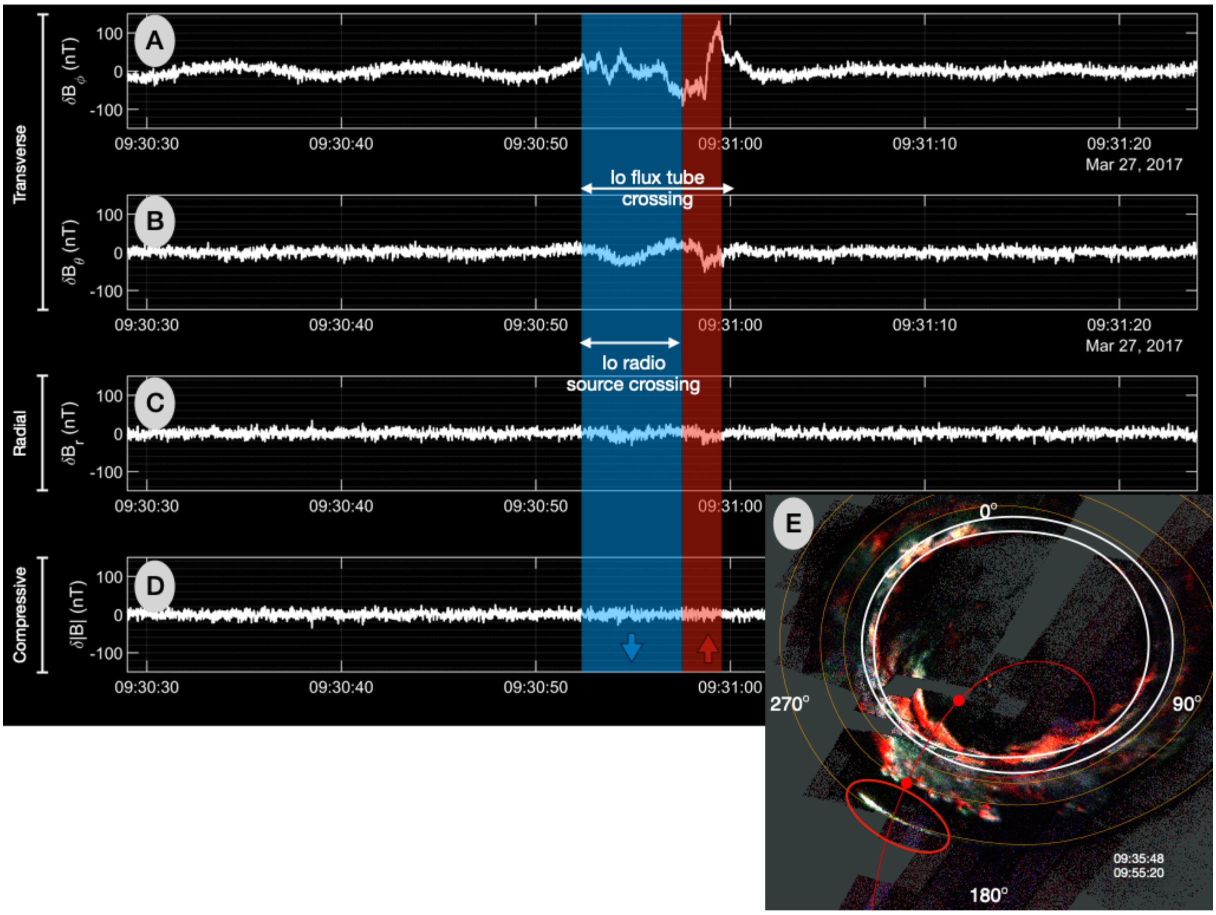


*Figure S1: Magnetic field perturbations (spherical coordinates) during Io-induced radio emission source crossing that occurs during Perijove #5 South (2017 March 27). Transverse perturbations: (A) $\delta B_\varphi$ and (B) $\delta B_\theta$; Radial perturbations: (C) $\delta B_r$; Compressive perturbations: (D) $\delta|B|$. The blue shaded area represents downward current, while the red area represents upward current.*

*Panel (E) shows the polar projection (as seen from the Southern pole) of Juno/UVS data with Juno's trajectory overplotted. The two red point shows the integrated time of the image (indicated on the bottom-right corner of the image). The red ellipse highlight the crossing of interest.*

**Figure S2 – Juno/ measurements during Io-induced radio emission source crossing on 2017 May 29 (Perijove #6 North)**

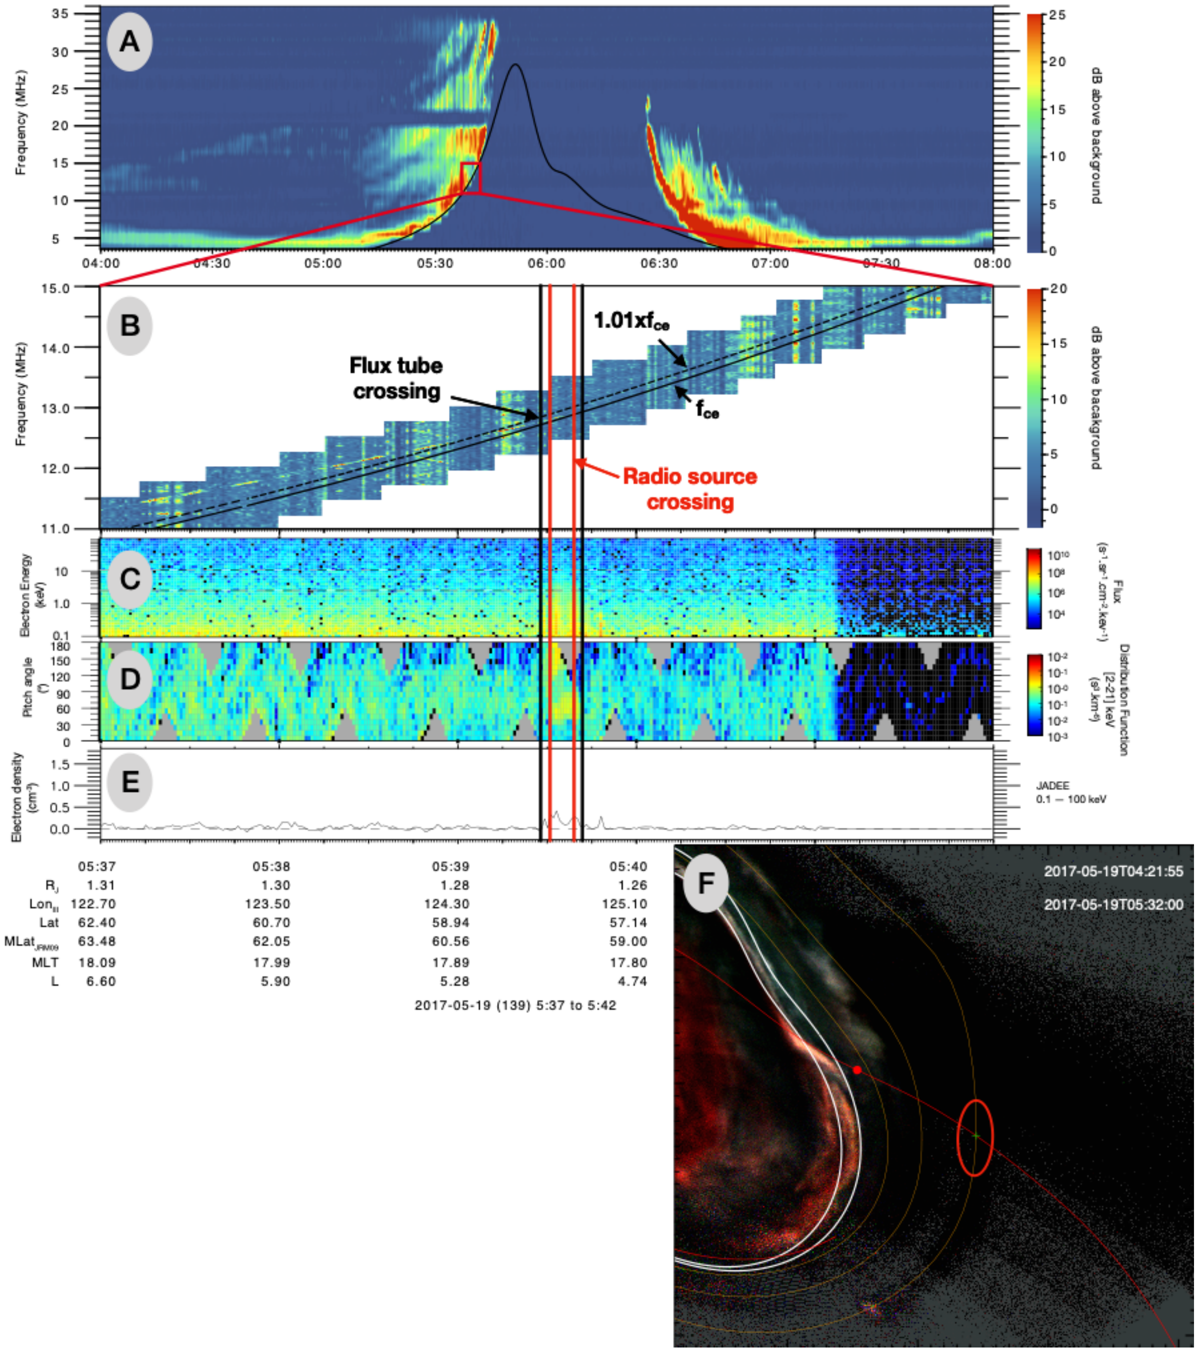


*Figure S2: Juno data during Perijove #6 North (2017 May 19), during an Io-induced radio emission source crossing. Panels (A,B) display Juno/Waves data (A) in low-resolution mode and (B) in high-resolution mode. The solid-black lines represent the electron cyclotron frequency derived from the magnetic field measurements of Juno/MAG, and the dashed-black line is 1.01x$f_{ce}$. Panels (C-E) display Juno/JADE-E measurements: (C) the electron differential number flux (or intensity) of all electrons; (D) the electron distribution function for energy in range [2-21] keV as a function of pitch angle; (E) partial electron density calculated from the JADE-E flux. The vertical solid black lines represent the flux tube crossing as inferred from JADE data, while vertical red lines represent the time interval where growth rate > $10^{-4}$ are calculated from JADE measurements. Panel (F) shows the polar projection (as seen from the Northern pole) of Juno/UVS data with Juno's trajectory*

*overplotted. The two red point shows the integrated time of the image (indicated on the top-right corner of the image). The red ellipse highlights the crossing of interest. Juno/MAG measurements show no significant magnetic field perturbation (potentially due to a very small electron density), and are therefore not shown.*

**Figure S3 – Juno/ measurements during Io-induced radio emission source crossing on 2020 September 16 (Perijove #29 North)**

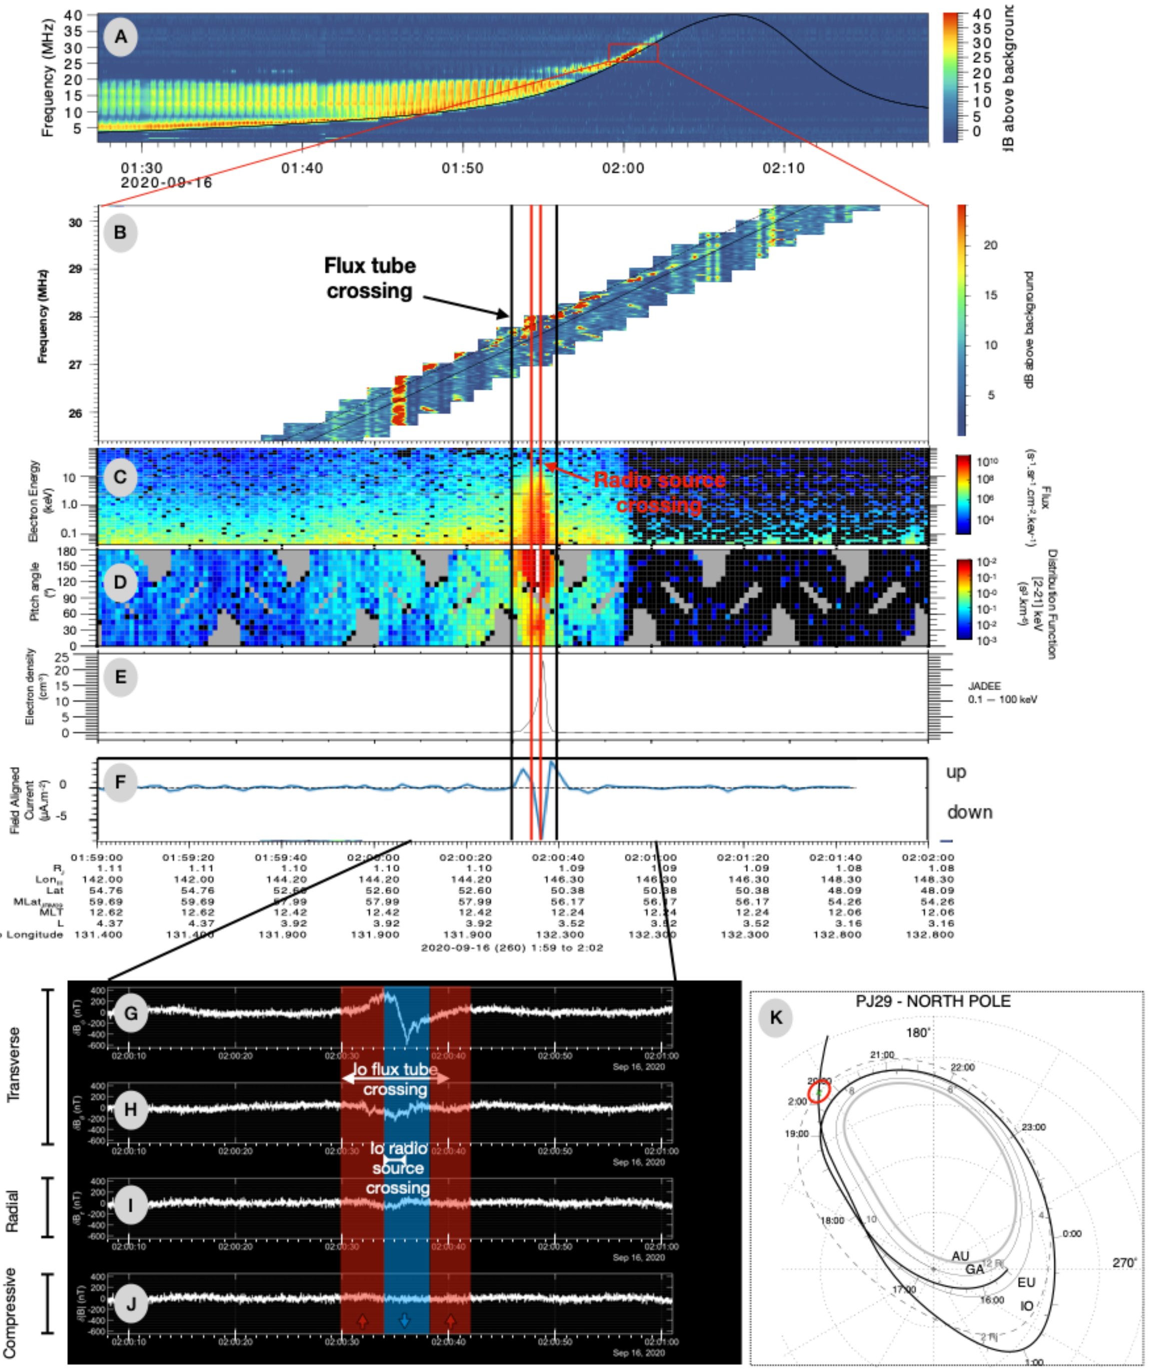


*Figure S3: Juno data during Perijove #29 North (2020 September 16), during an Io-induced radio emission source crossing. Panels (A,B) display Juno/Waves data (A) in low-resolution mode and (B) in high-resolution mode. The solid-black lines represent the electron cyclotron frequency derived from the magnetic field measurements of Juno/MAG, and the dashed-black line is 1.01x$f_{ce}$. Panels (C-E) display Juno/JADE-E measurements: (C) the electron*

*differential number flux (or intensity) of all electrons; (D) the electron distribution function for energy in range [2-21] keV as a function of pitch angle; (E) partial electron density calculated from the JADE-E flux. Panel (F) shows the field aligned currents calculated based on Al Saati et al. (2022)'s method, using magnetic field fluctuations in the azimuthal direction ($\delta B_\varphi$) deduced from the Juno/MAG measurements.*
*The vertical solid black lines represent the flux tube crossing as inferred from JADE data, while vertical solid red lines represent the time interval where growth rate > $10^{-4}$ are calculated from JADE measurements.*
*Panels (G-J): Magnetic field perturbations (spherical coordinates) from Juno/MAG measurements: Transverse perturbations: (G) $\delta B_\varphi$ and (H) $\delta B_\theta$; Radial perturbations: (I) $\delta B_r$; Compressive perturbations: (J) $\delta|B|$. The blue shaded area represents downward current, while the red areas represent upward currents.*
*Panel (K) shows the polar projection of Juno's trajectory (as seen from the Northern pole). The red ellipse highlights the position of Juno at the crossing time. Not enough Juno/UVS data were available for this crossing to build a UV map of context.*

**Figure S4 – Juno/ measurements during Io-induced radio emission source crossing on 2017 March 17 (Perijove #5 North)**

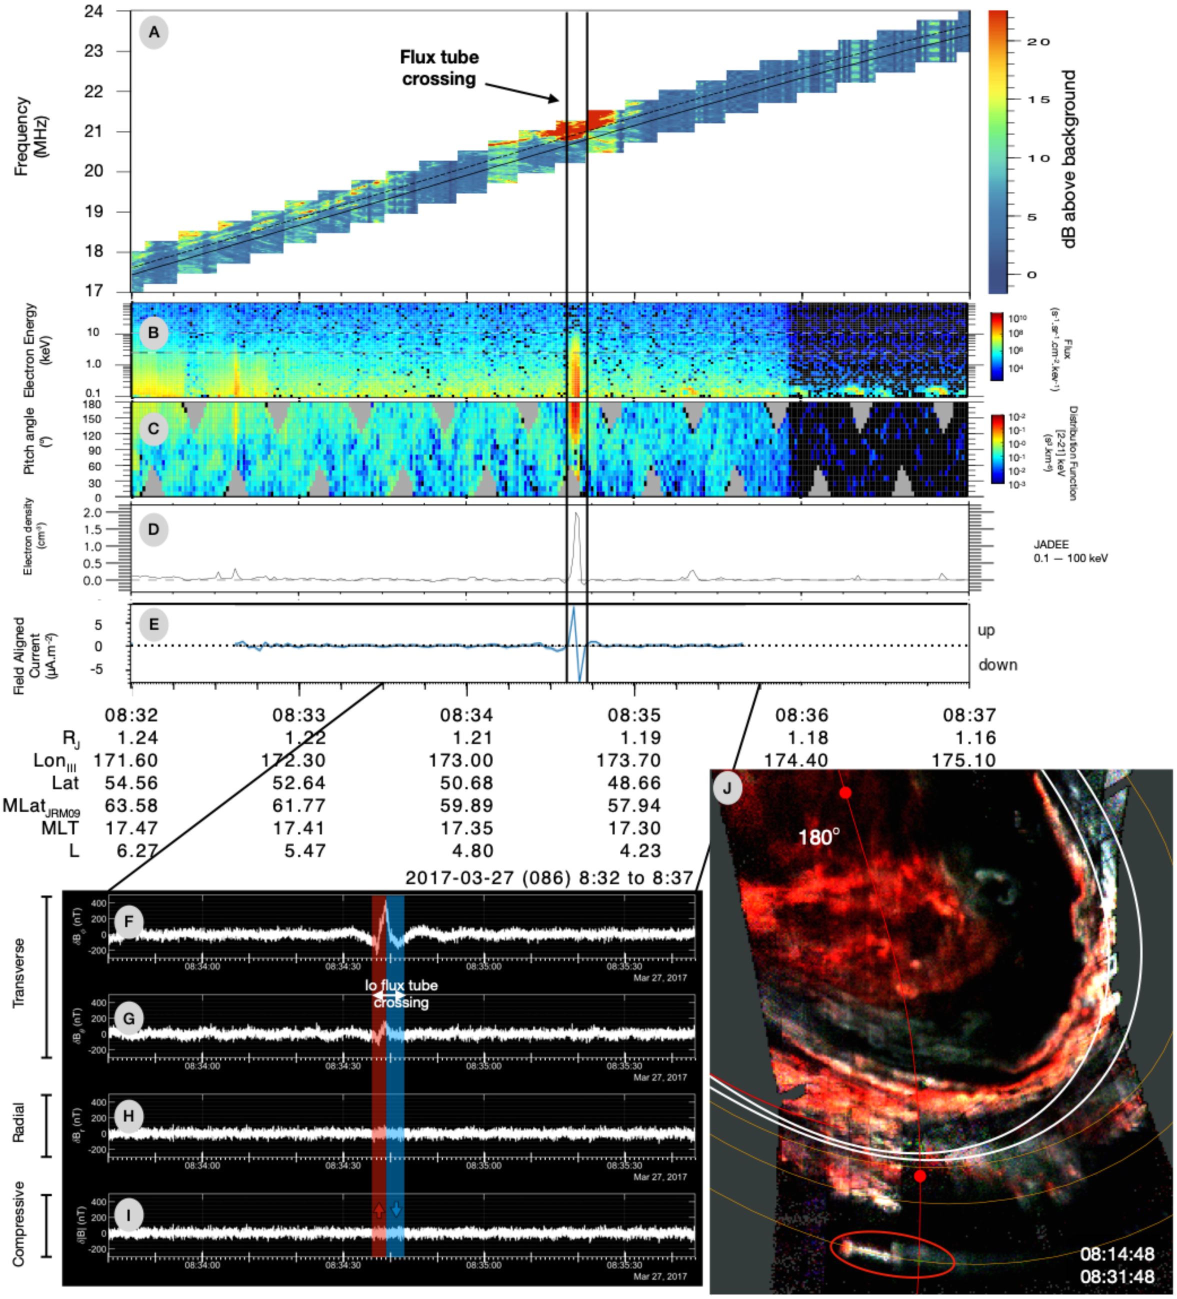


*Figure S4: Juno data during Perijove #5 North (2017 March 17), during an Io-induced radio emission source crossing. Panel (A) displays Juno/Waves data in high-resolution mode. The solid-black lines represent the electron cyclotron frequency derived from the magnetic field measurements of Juno/MAG, and the dashed-black line is 1.01x$f_{ce}$. Panels (B-D) display Juno/JADE-E measurements: (B) the electron differential number flux (or intensity) of all electrons; (C) the electron distribution function for energy in range [2-21] keV as a function of pitch angle; (D) partial electron density calculated from the JADE-E flux. Panel (E) shows the field aligned currents calculated based on Al Saati et al. (2022)'s method, using magnetic field fluctuations in the azimuthal direction ($\delta B_\varphi$) deduced from the Juno/MAG measurements. The vertical solid black lines represent the flux tube crossing as inferred from JADE data. Panels (F-I): Magnetic field perturbations (spherical coordinates) from Juno/MAG measurements: Transverse perturbations: (F) $\delta B_\varphi$ and (G) $\delta B_\theta$; Radial perturbations: (H)*

*$\delta B_r$; Compressive perturbations: (I) $\delta|B|$. The blue shaded area represents downward current, while the red area represents upward current.*
*Panel (J) shows the polar projection (as seen from the Northern pole) of Juno/UVS data with Juno's trajectory overplotted. The two red point shows the integrated time of the image (indicated on the bottom-right corner of the image). The red ellipse highlights the crossing of interest.*

**Figure S5 – Magnetic field perturbations from Juno/MAG measurements during Ganymede-induced radio emission source crossing on 2019 May 29 (Perijove #20 North)**

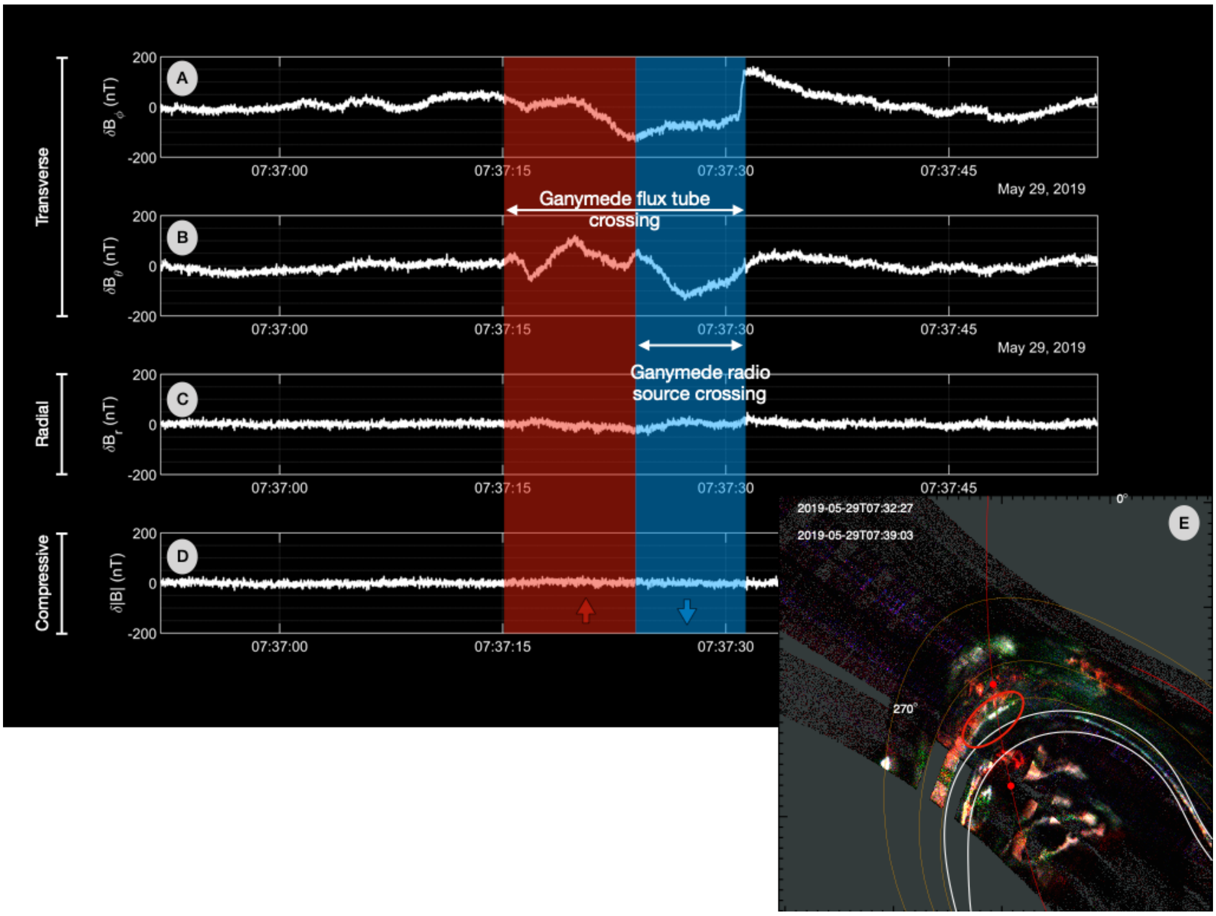


*Figure S5: Magnetic field perturbations (spherical coordinates) during Ganymede-induced radio emission source crossing that occurs during Perijove #20 North (2019 May 29). Transverse perturbations: (A) $\delta B_\varphi$ and (B) $\delta B_\theta$; Radial perturbations: (C) $\delta B_r$; Compressive perturbations: (D) $\delta|B|$. The blue shaded area represents downward current, while the red area represents upward current. Panel (E) shows the polar projection (as seen from the Northern pole) of Juno/UVS data with Juno's trajectory overplotted. The two red point shows the integrated time of the image (indicated on the top-right corner of the image). The red ellipse highlights the crossing of interest.*
